# Supplementary material for: Multiple Instance Neural Networks Based on Sparse Attention for Cancer Detection using T-cell Receptor Sequences
Source: arXiv:2208.04524 source file (2022-08-09)
Supplement: Supplementary file 1 [file appendix.tex]

In Figure \ref{fig:extracted}, extracted features of bags are illustrated in heatmap. The heatmap is given in a $n \times p$ matrix form with colored in blue-yellow spectrum. The figure shows that the extracted features using the sparsemax case are more activated than using the softmax case. Hence, the difference between features in each observation of sparsemax case is larger than softmax case. The results demonstrate that the extracted features from sparsemax are more appropriate to characterize the property of each instance. We believe that the sparsity in the proposed attention structure selects important features merged to discriminate bags accurately in the classification layer.

\begin{figure}[htp]
	\centering
%	\begin{minipage}{0.5\linewidth}
		\includegraphics[page=1,width=1\linewidth]{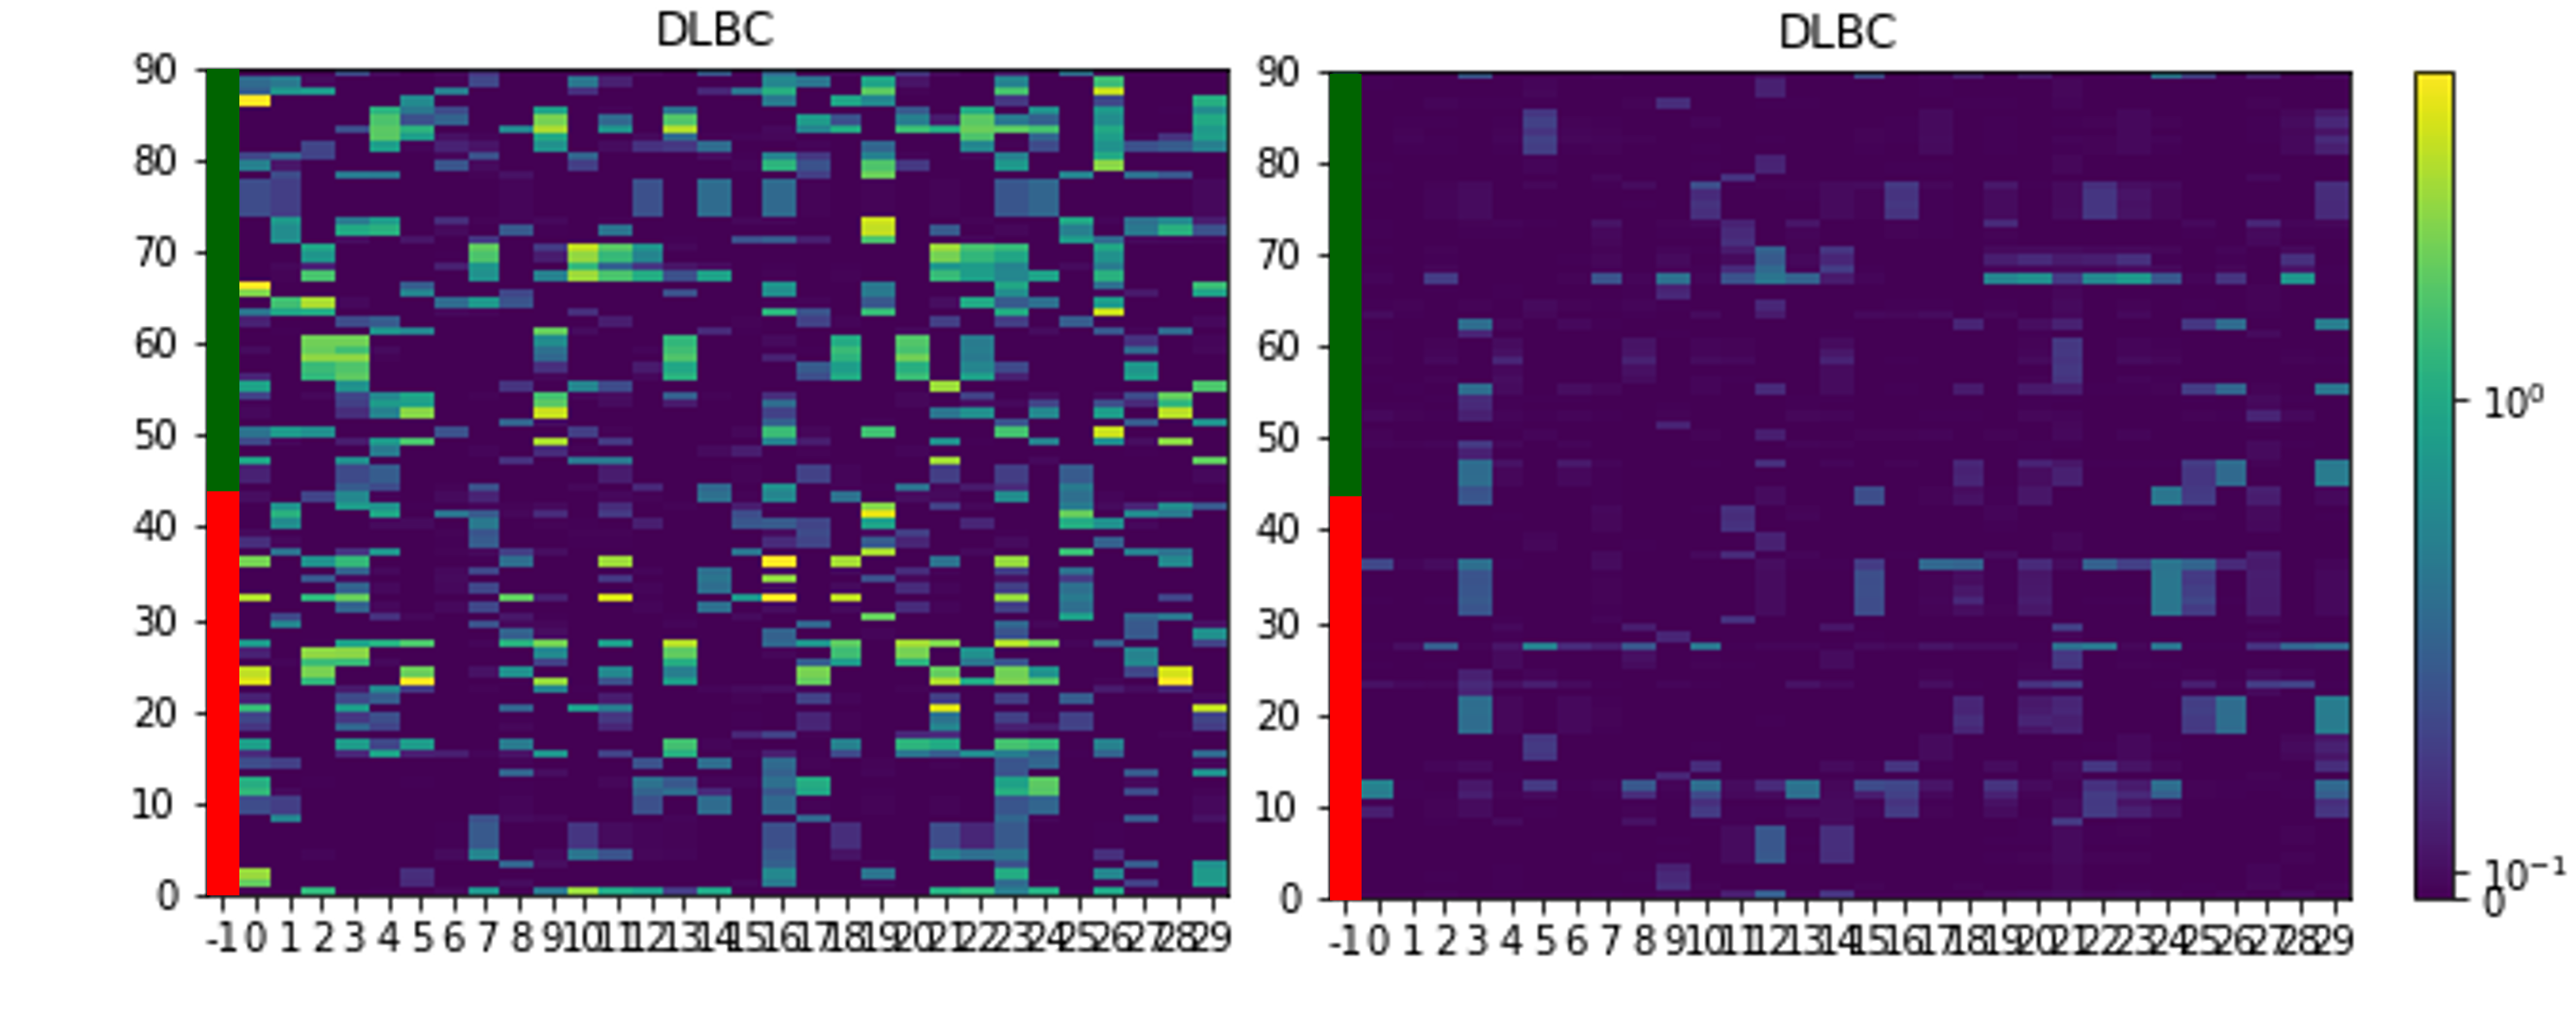}
		
%	\end{minipage}
	\caption{Heatmap of extracted features via the sparsemax (left) and softmax (right) function. Values are min-max normalized and transformed in log-scale. Red and green labels indicate tumor and normal samples, respectively. Here, we show the balanced case for DLBC cancer data.}
	\label{fig:extracted}
\end{figure}
